# Supplementary material for: Learning to Segment Actions from Observation and Narration
Source: arXiv:2005.03684 source file (2020-08-12)
Supplement: Supplementary file 1 [file 06e-results-supp.tex]

\input{06c-results-oracle-background-unsup.tex}

\subsection{Narration as Features}
\df{possibly reorder these sections, if we're able to get the DM results with narration in Zhukov's model in time, and use final numbers from that}

We found that, when used to define hard constraints on inference during training time (as in \citet{zhukov2019cross}), video narration substantially improves performance. We now experiment with adding it as a feature both during training and testing, to allow the model to learn to condition on it. We obtain a vector $v_t$ for each timestep $t$ in a window by averaging word vectors from the transcribed naration within a \red{XX} second window around $t$, then apply PCA as in \Section{sec:feature_models}, and concatenate with the other PCA-reduced features (I3D, ResNet, and audio) to produce the vectors $x_t$. Training and evaluating the model then proceeds as before. \Table{tbl:narration} shows that adding in these narration features produces reliable improvements in the models, although the relative gains are not so large as the gains obtained from adding narration constraints during inference.\footnote{
We conjecture that the hard constraints benefit from the similarities \citet{zhukov2019cross} computed between step labels and the narration vectors. Incorporating these into the generative model in a soft way is an interesting direction for future work. \df{if time, actually do this}
}

\begin{table}[h]
\small{
\begin{tabular}{lcc|cc}
    \toprule
    & \multicolumn{2}{c}{Step Frame F1} & \multicolumn{2}{c}{Step Recovery}  \\
    & No Narr & w/ Narr. & No Narr & w/ Narr \\
    \midrule
\multicolumn{5}{l}{\bf Supervised} \\
Gaussian Mixture & 40.9 & 43.7 & 31.5 & 34.9 \\
HSMM & 49.7 & 53.2 & 28.7 & 32.1 \\
\zhukov & 18.0 & \red{??} & 45.3 & \red{??} \\ %
    \midrule
\multicolumn{5}{l}{\bf Weakly Supervised} \\
HSMM & 31.8 & \red{running} & 10.6 & \red{running} \\
HSMM+Narr & 9.8 & 8.0 & 8.5 & 12.6  \\
HSMM+Order & 8.4 & 9.5 & 7.3 & 8.5  \\
HSMM+Ord+Narr & 16.1 & 17.9 & 17.2 & 21.9  \\
\zhukov & 1.8 & \red{??} & 24.5 & \red{??} \\ %
\bottomrule
\end{tabular}
}
\caption{\label{tbl:narration}Effects of adding narration features. \df{?? results would need to be obtained at DM. Consider just reporting full models for the weakly supervised setting (take out HSMM,HSMM+Narr,HSMM+Order.} }
\end{table}

\input{06d-results-final.tex}
